# Supplementary material for: Delving into Multimodal Prompting for Fine-grained Visual Classification
Source: arXiv:2309.08912 source file (2023-12-13)
Supplement: Supplementary file 1 [file appendix.tex]

\section{Appendix}
\subsection{Influence of the number of selected tokens.} The performance comparison of different token selection numbers $K$  in \textsc{CsVP} are depicted in Fig.~\ref{fig:select_number}. We observed that performance degrades when the $K$ exceeds 14. The reason for the performance drop may be that as the number of selected tokens increases, the model may select tokens that mislead the classification. For this, we set $K$ to 14 on all datasets.
\begin{table}[H]
    \centering
    \begin{tabular}{l|c|c}
    \hline
         Position &CUB &NABirds  \\
         \hline
         $l=L-3$ &90.0 &89.3 \\
         $l=L-2$ &91.0 &90.6 \\
         $l=L-1$ &\textbf{91.8} &\textbf{91.0} \\
         \hline
    \end{tabular}
    \caption{Accuracy~(\%) comparison of different insertion positions for the semantic token selection module on CUB-200-2011 and NABirds.}
    \label{tab:tsm_layer}
    \vspace{-4mm}
\end{table}

\subsection{Influence of the \textsc{CsVP} insert position.} The results of the different  insert position of \textsc{CsVP} are shown in Table~\ref{tab:tsm_layer}. We find that the deeper the block inserted by \textsc{CsVP}, the better the performance. This is likely because self-attention in deeper blocks is more semantic, enabling a more precise selection of discriminative tokens. Based on the above observations, we insert the \textsc{CsVP} at the $(L-1)$-th block in all our experiments.

\subsection{Why the VLFM works.} In this part, we perform a comprehensive analysis of the different components comprising the VLFM. Following the completion of the first stage of training, the textual features of each subcategory exhibit high similarity to the visual features of the corresponding subcategory due to the optimization of the textual features through contrastive learning. Consequently, we perform experiments to compute the similarity between textual features and visual features for subcategory prediction. As shown in Table~\ref{tab:cos_sim}, we have noted a considerable decline in performance when employing similarity prediction. The likely reason for this is the presence of noise between textual features and visual features, and the utilization of similarity calculations for predictions fails to eliminate it. While LAI utilizes VLFM to extract valuable semantic information from textual features and enhance visual features. Then, to demonstrate the role of cross-attention in VLFM for extracting semantic information from textual features, we compared it with self-attention applied solely to visual features. From the results in Table~\ref{tab:self_cross}, we can observe that computing self-attention solely on visual features has no effect, indicating that our VLFM module effectively extracts valuable semantic information from textual features using cross-attention. 

\begin{table}
    \centering
    \begin{tabular}{c|c|c}
    \hline
        Method &CUB &NABirds \\
        \hline
         Similarity & 90.9 & 90.0 \\
         MPF & \textbf{91.8} & \textbf{91.0} \\
         \hline
    \end{tabular}
    \caption{Comparison results of similarity prediction and MPF on CUB-200-2011 and NABirds.}
    \label{tab:cos_sim}
\end{table}
\begin{table}
    \centering
    \begin{tabular}{c|c|c}
    \hline
        Setting &CUB &NABirds \\
        \hline
        Without VLFM & 91.5 & 90.8 \\
         Self-attention & 91.5 & 90.8 \\
         Cross-attention & \textbf{91.8} & \textbf{91.0} \\
         \hline
    \end{tabular}
    \caption{Accuracy~(\%) comparison results with various VLFM settings on CUB-200-2011 and NABirds.}
    \label{tab:self_cross}
\end{table}
